# Supplementary material for: Masked Label Prediction: Unified Message Passing Model for Semi-Supervised Classification
Source: arXiv:2009.03509 source file (2021-05-10)
Supplement: Supplementary file 1 [file appendix.tex]

\appendix
\begin{appendices}
\section{Datasets Details}
{\bf ogbn-products.} As shown in Table \ref{table:ogb}, \emph{ogb-products} is an undirected and unweighted graph, representing an Amazon product co-purchasing network. The goal of this task is to predict the category of a product in a multi-class classification setup, where the 47 top-level categories are used for target labels. To match the real-world application, it conducts a splitting on the dataset based on sales ranking, where the top 10\% for training, next top 2\% for validation, and the rest for testing.

{\bf ogbn-proteins.} As shown in Table \ref{table:ogb}, \emph{ogbn-proteins} dataset is an undirected, weighted, and typed (according to species) graph. Nodes represent proteins, and edges indicate different types of biologically meaningful associations between proteins, e.g., physical interactions, co-expression or homology. The task is to predict the presence of protein functions in a multi-label binary classification setup, where there are 112 kinds of labels to predict in total. The performance is measured by the average of ROC-AUC scores across the 112 tasks. It conducts the splitting by species.

{\bf ogbn-arxiv.} As shown in Table \ref{table:ogb}, \emph{ogbn-arxiv} dataset is a directed graph, representing the citation network between all Computer Science (CS) arXiv papers indexed by MAG \citep{wang2020microsoft}. The task is to predict the 40 subject areas of arXiv CS papers, e.g., cs.AI, cs.LG, and cs.OS, which are manually determined by the paper’s authors and arXiv moderators. This dataset were splitted by time.
\label{appendix:dataset}

\section{ hyper-parameters tuned on UniMP model}
There are the hyper-parameters we tuned on our unified model for comparison with other SOTA results, where the asterisks denote the hyper-parameters we eventually selected.

\begin{table}[htbp]
\caption{The tuned hyperparamerters of our model}
\begin{tabular}{cccc}
\hline
                 & \textbf{ogbn-prdouct} & \textbf{ogbn-proteins}   & \textbf{ogbn-arxiv}                                                                          \\ \hline
sampling\_method & NeighborSampling      & Random Partition         & Full-batch                                                                                   \\ \hline
num\_layers      & {[}3*, 4{]}           & {[}3, 5, 7*, 9{]}        & {[}3*, 4{]}                                                                                  \\ \hline
hidden\_size     & {[}128*, 256{]}       & {[}32, 64*, 128{]}       & {[}128*, 256{]}                                                                              \\ \hline
num\_heads       & {[}4*,2{]}            & {[}6, 4*, 2{]}           & {[}2*, 1{]}                                                                                  \\ \hline
dropout          & {[}0.3*{]}            & {[}0, 0.1*, 0.3{]}       & {[}0.1, 0.3*{]}                                                                              \\ \hline
lr               & {[}0.01, 0.001*{]}    & {[}0.01, 0.001*{]}       & {[}0.1, 0.001*{]}                                                                            \\ \hline
weight\_decay    & -                     & -                        & {[}0, 0.0005*{]}                                                                             \\ \hline
label\_rate      & {[}0.625*{]}          & {[}0.375, 0.5*, 0.625{]} & \begin{tabular}[c]{@{}c@{}}{[}0.125, 0.25, 0.375, 0.5,\\ 0.625*, 0.75, 0.875{]}\end{tabular} \\ \hline
\end{tabular}
\end{table}
\label{appendix:hyp_sota}
\end{appendices}
