# Supplementary material for: Masked Label Prediction: Unified Message Passing Model for Semi-Supervised Classification
Source: arXiv:2009.03509 source file (2021-05-10)
Supplement: Supplementary file 3 [file get_appendix.tex]

\documentclass[a4paper]{article}
\usepackage{pdfpages}
\usepackage{graphicx}
\begin{document}
\includepdfmerge{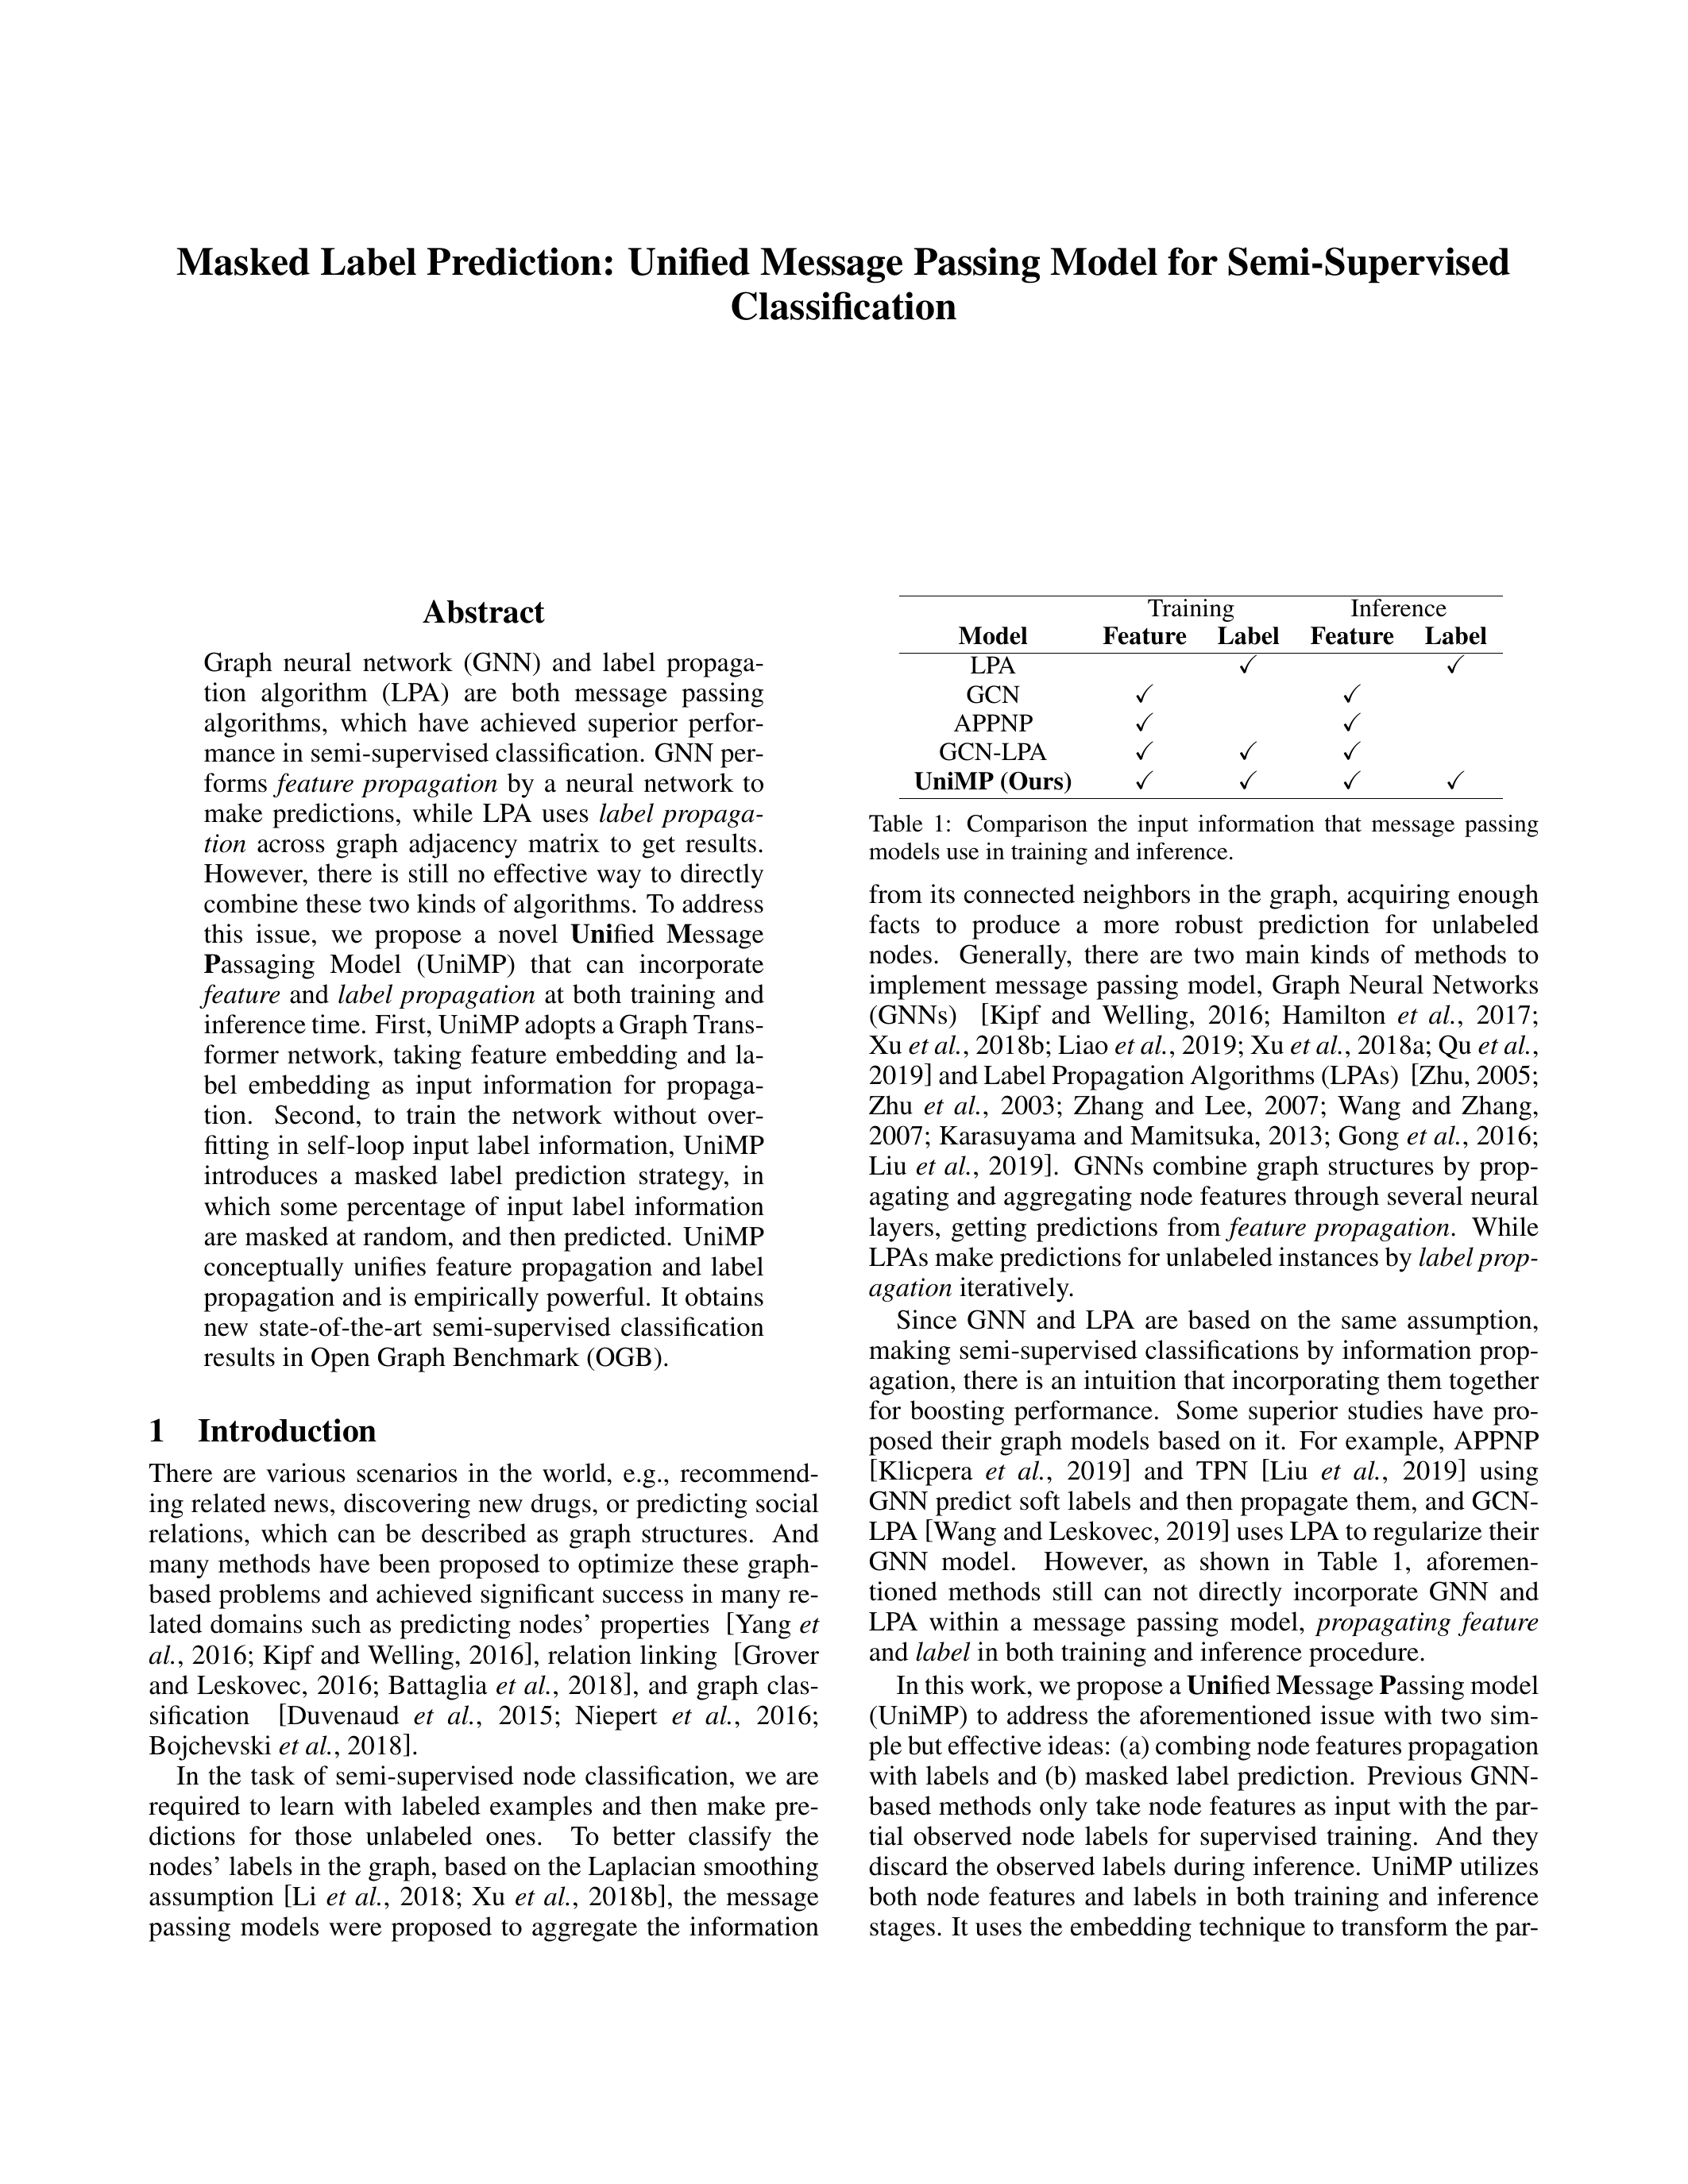,9}
\end{document}
